# Supplementary material for: Generalization by Adaptation: Diffusion-Based Domain Extension for Domain-Generalized Semantic Segmentation
Source: arXiv:2312.01850 source file (2023-12-04)
Supplement: Supplementary file 2 [file supplement_synthia_visv2.tex]

\documentclass{standalone}
\usepackage{graphicx}
\usepackage{tikz}
\usetikzlibrary{positioning}

\begin{document}
\graphicspath{{./fig}{../fig}}
\makeatletter
  \newcommand\tinyv{\@setfontsize\tinyv{2pt}{6}}
\makeatother
\def\x{4.3cm}  
\def\y{3.6cm} 
\def\shift{4.5cm}  

\def\z{4.1cm} 
\def\r{4.4cm} 
\begin{tikzpicture}[
 ] 
 \setlength{\baselineskip}{4pt}
\node at (0,0) (frame1)
    {\includegraphics[width=\z]{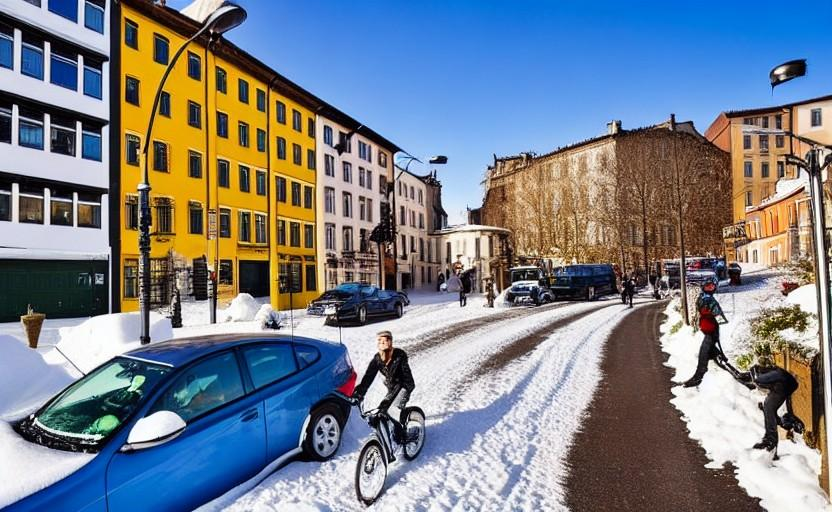}};
\node[left of= frame1, node distance=4.5cm] (frame4)
    {\includegraphics[width=\r]{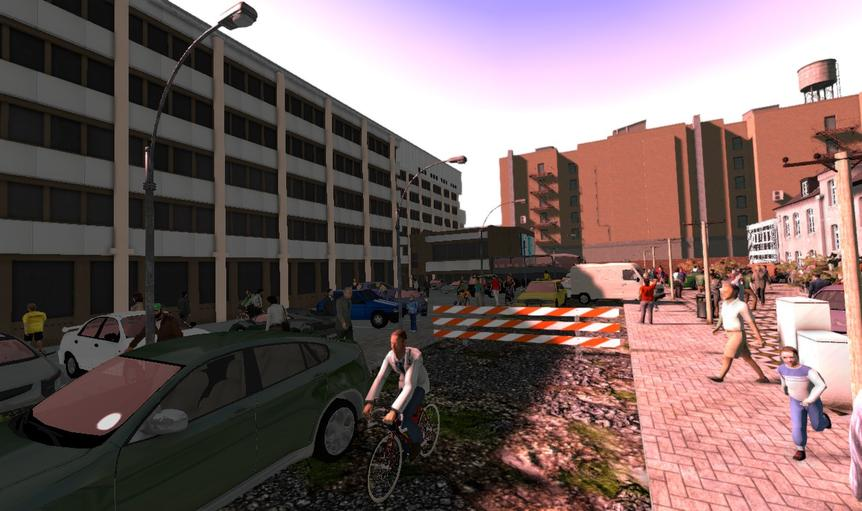}};
\node[right of= frame1, node distance=\x] (frame7)
    {\includegraphics[width=\z]{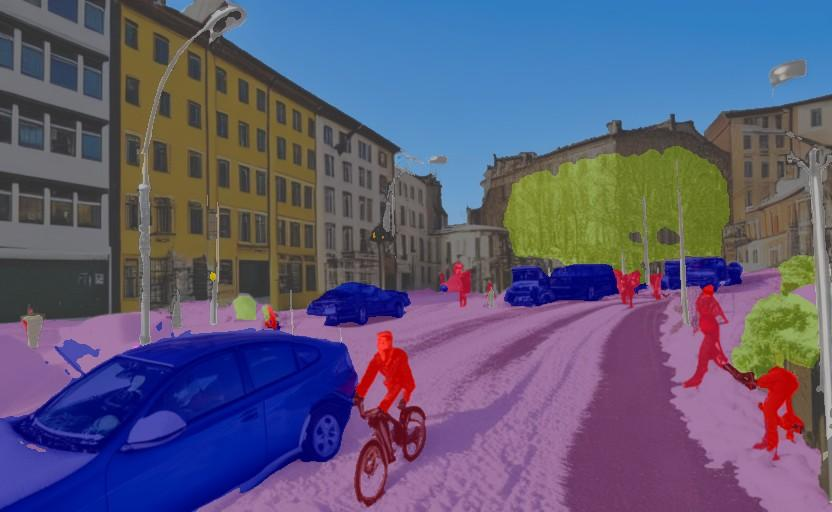}};
\node [above of=frame1, xshift=-0.2cm, node distance=1.8cm, text width=14cm, execute at begin node=\setlength{\baselineskip}{4pt}, draw, color=black](tex1){\footnotesize $\boldsymbol{\Phi}_n\!=$"\textit{A high quality photo; Europe; terrain, road, sidewalk, building, wall, fence, pole, vegetation, sky, person, rider, car, bus, motorcycle, bicycle, snowy}"} ;

\node[below of=frame1, node distance=\y] (frame8)
    {\includegraphics[width=\z]{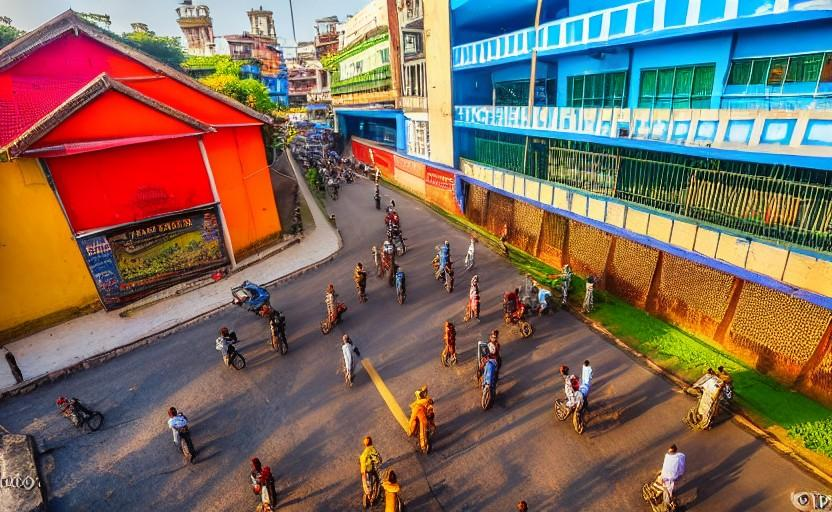}};
\node[below of= frame4, node distance=\y] (frame9)
    {\includegraphics[width=\r]{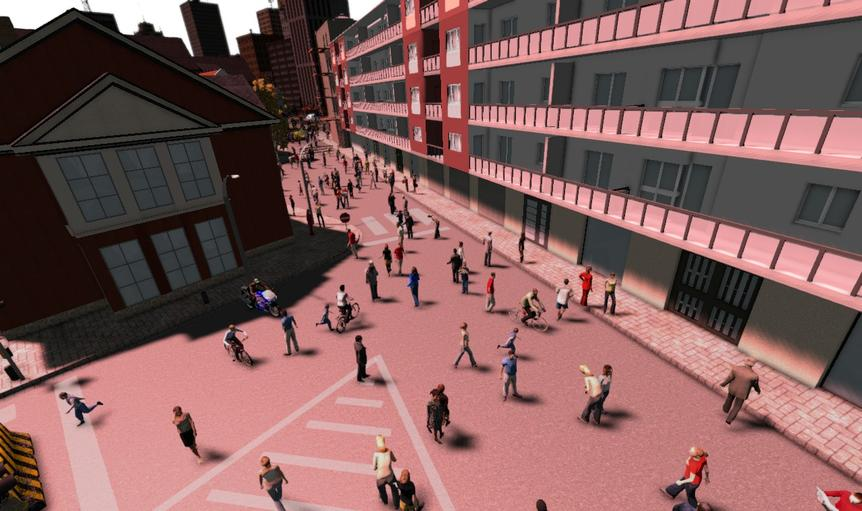}};
\node[below of= frame7, node distance=\y] (frame10)
    {\includegraphics[width=\z]{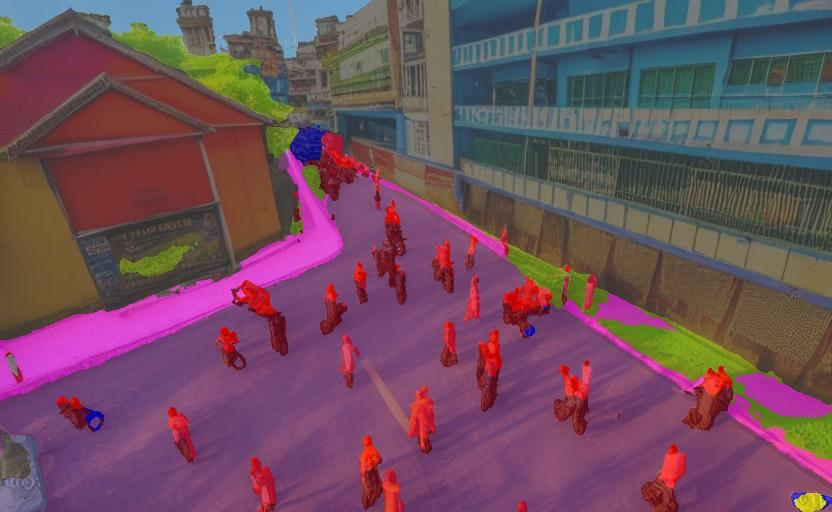}};
\node [above of=frame8, xshift=-0.2cm, node distance=1.8cm, text width=14cm, execute at begin node=\setlength{\baselineskip}{4pt}, draw, color=black](tex1){\footnotesize $\boldsymbol{\Phi}_n\!=$"\textit{A high quality photo; India; Highway, truck, road, sidewalk, building, fence, pole, traffic light, traffic sign, vegetation, sky, person, rider, car, motorcycle, bicycle, spring}"} ;

\node[below of=frame8, node distance=\y] (frame11)
    {\includegraphics[width=\z]{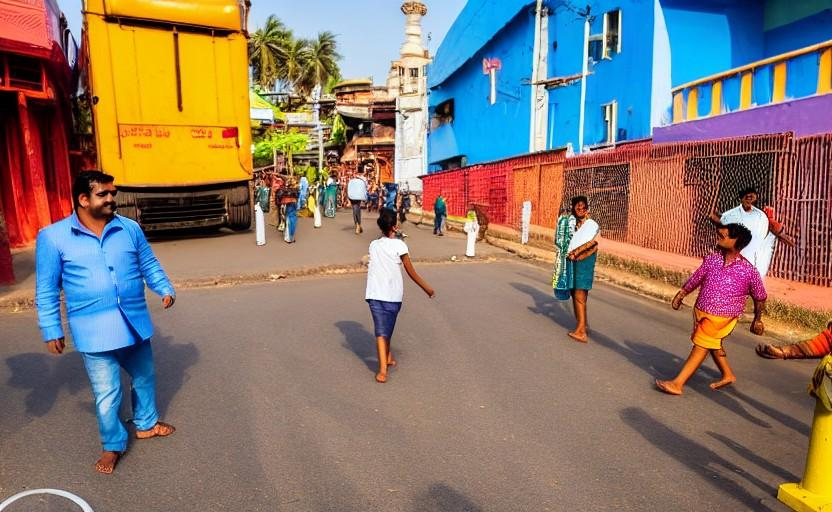}};
\node[below of= frame9, node distance=\y] (frame12)
    {\includegraphics[width=\r]{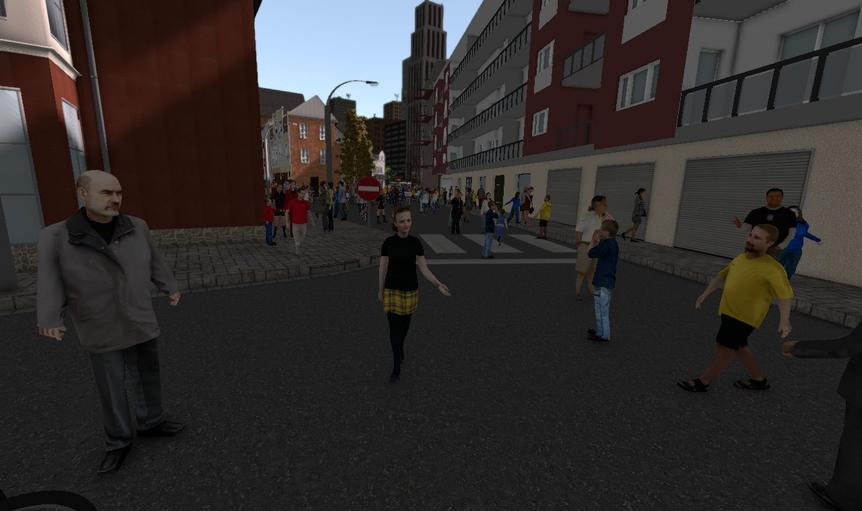}};
\node[below of= frame10, node distance=\y] (frame13)
    {\includegraphics[width=\z]{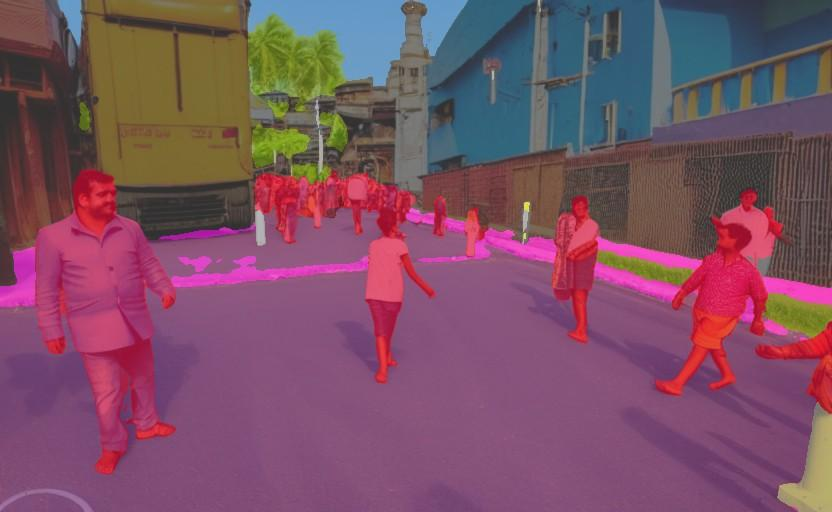}};
\node [above of=frame11, xshift=-0.2cm, node distance=1.8cm, text width=14cm, execute at begin node=\setlength{\baselineskip}{4pt}, draw, color=black](tex1){\footnotesize $\boldsymbol{\Phi}_n\!=$"\textit{A high quality photo; India; truck, road, sidewalk, building, fence, pole, traffic light, traffic sign, vegetation, sky, person, rider, car, bus, motorcycle, bicycle, sunny}"} ;

\node[below of=frame11, node distance=\y] (frame14)
    {\includegraphics[width=\z]{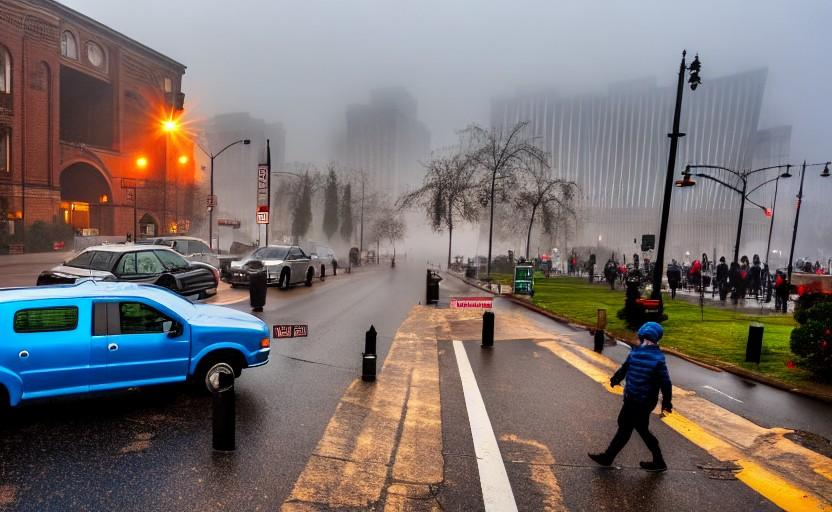}};
\node[below of= frame12, node distance=\y] (frame15)
    {\includegraphics[width=\r]{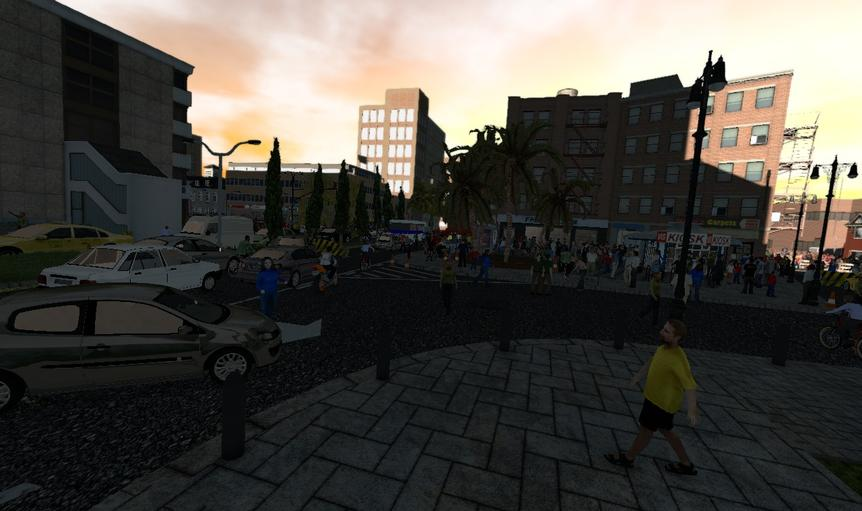}};
\node[below of= frame13, node distance=\y] (frame16)
    {\includegraphics[width=\z]{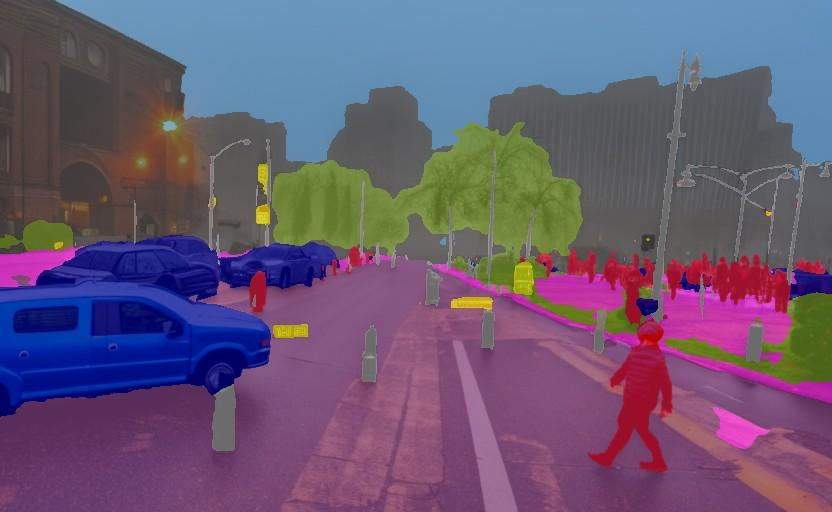}};
\node [above of=frame14, xshift=-0.2cm, node distance=1.8cm, text width=14cm, execute at begin node=\setlength{\baselineskip}{4pt}, draw, color=black](tex1){\footnotesize $\boldsymbol{\Phi}_n\!=$"\textit{A high quality photo; USA; City, truck, road, sidewalk, building, wall, fence, pole, traffic light, traffic sign, vegetation, sky, person, rider, car, bus, motorcycle, bicycle, fog/mist}"} ;

\node[below of=frame14, node distance=\y] (frame17)
    {\includegraphics[width=\z]{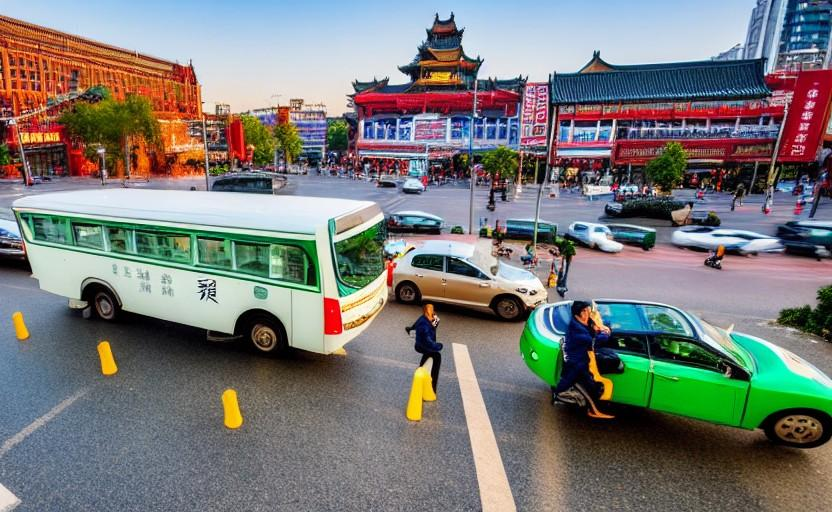}};
\node[below of= frame15, node distance=\y] (frame18)
    {\includegraphics[width=\r]{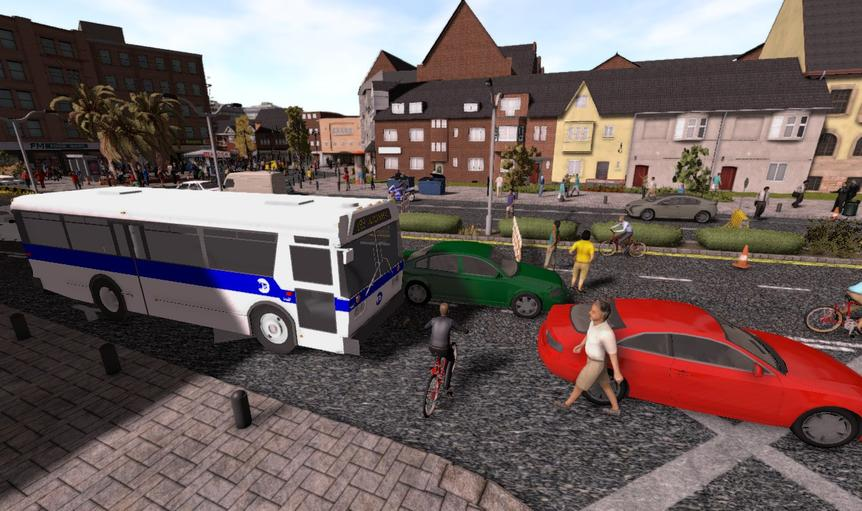}};
\node[below of= frame16, node distance=\y] (frame19)
    {\includegraphics[width=\z]{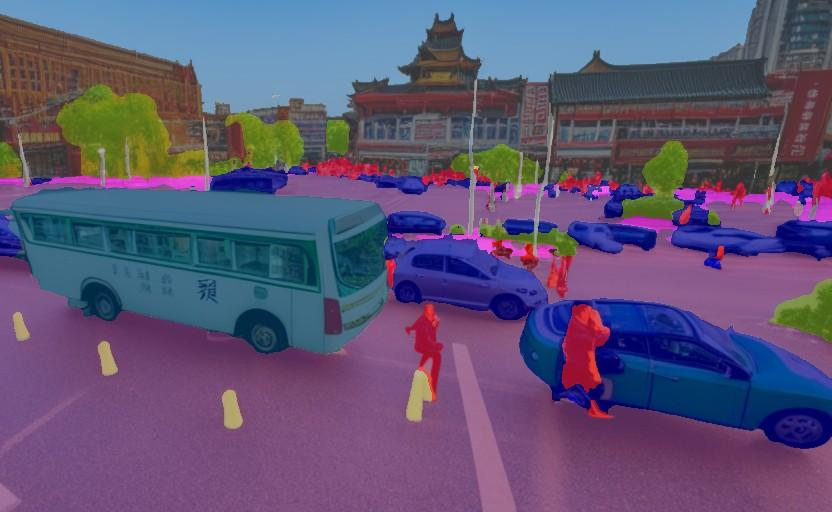}};
\node [above of=frame17, xshift=-0.2cm, node distance=1.8cm, text width=14cm, execute at begin node=\setlength{\baselineskip}{4pt}, draw, color=black](tex1){\footnotesize $\boldsymbol{\Phi}_n\!=$"\textit{A high quality photo; China; city, terrain, road, sidewalk, building, fence, pole, traffic light, traffic sign, vegetation, sky, person, rider, car, bus, motorcycle, bicycle, morning}"} ;

\node [above of=frame4, node distance=2.8cm](tex1){ \small\textsf{\textbf{GTA5 Input $\mathbf{x}_n^{\mathrm{S}}$}}} ;
 \node [above of=frame1, node distance=2.8cm](tex1){\small\textsf{\textbf{Diffusion Sample $\mathbf{x}_n^{\mathrm{PT}}$}}} ;
 \node [above of=frame7, node distance=2.8cm](tex1){ \small\textsf{\textbf{Prediction $\VEC{M}^\mathrm{DG}(\mathbf{x}_n^{\mathrm{PT}})$}}} ;
\end{tikzpicture}
\end{document}
